# Supplementary material for: The Lean Data Scientist: Recent Advances towards Overcoming the Data Bottleneck
Source: arXiv:2211.07959 source file (2022-11-15)
Supplement: Supplementary file 1 [file appendix.tex]

\newpage
\section{}

\subsection{}

\begin{table*}
\begin{tabular}{|c|c|c|}
\hline 
 Obstacle & Solution & Methods \\ 
 \hline
 \multirow{3}{*}{Not enough data} & Data recycling \& generation &
    \begin{minipage}[t]{0.3\textwidth} 
        \begin{itemize}
            \item \textbf{Dataset reusing: }Reuse a dataset for a different purpose from the one it was originally constructed for.
             \item \textbf{Data augmentation: }Perform reasonable transformations on $\mathcal{X}$ enlarge the dataset (and prevent overfitting).
             \item \textbf{Active learning:} Generate ``near-miss'' examples, which are close to the decision boundary. Considered to contribute more to the learning process than a random example.
         \end{itemize}
     \end{minipage}\\ \cline{2-3}
 {} & Utilizing additional information on $\mathcal{X}$ &
    \begin{minipage}[t]{0.3\textwidth} 
        \begin{itemize}
             \item \textbf{Multimodal learning:} Enrich the learning process by integrating associated information on $\mathcal{X}$ from multiple modalities.
             \item \textbf{Curriculum learning: }Present examples according to a predetermined, usually difficulty-based, curriculum.
         \end{itemize}
     \end{minipage}\\ \cline{2-3}
 {} & Models that can generalize & 
    \begin{minipage}[t]{0.3\textwidth} 
        \begin{itemize}
             \item \textbf{Multi-task learning: }Co-learn multiple tasks simultaneously to enhance their cross task similarities for better generalization ability.
             \item \textbf{Transfer learning: }Transfer knowledge gained while solving one problem to a different but related problem.
             \item \textbf{Meta learning: }Improve the learning algorithm by generalizing based on experience from multiple learning episodes
             \item \textbf{Few-shot learning: }Feeding the learner with only a few target specific data points, contrary to the standard data-abundant paradigm.
         \end{itemize}
     \end{minipage}\\  
 \hline
 \multirow{2}{*}{Labels for the abundant data} & Assuming constraints on $P(\mathcal{Y}=y|\mathcal{X}=x)$ & 
     \begin{minipage}[t]{0.3\textwidth} 
        \begin{itemize}
             \item \textbf{Semi-supervised learning:} Harness information regarding $P(\mathcal{X}=x)$ to reduce labeling requirements by integrating labeled and non-labeled examples in the learning process.
             \item \textbf{Data programming: }Integrate multiple weak heuristics regarding the labeling process $f: \mathcal{X} \xrightarrow{} \mathcal{Y}$ to create noisy labels. 
             \item \textbf{Expectation estimation: }Using prior regarding the proportion of the different labels in sub-groups of the data to create noisy labels.
         \end{itemize}
     \end{minipage}\\  \cline{2-3}
 {} & Supervision signal from external datasets & 
     \begin{minipage}[t]{0.3\textwidth} 
        \begin{itemize}
             \item \textbf{Incidental supervision: }Exploit weak signals that exist in data independently of the task at hand.
             \item \textbf{Distant supervision: }Utilize a preexisting database to collect examples for the desired relation. These examples are then used to automatically generate labeled training data.
         \end{itemize}
     \end{minipage}\\
 \hline
\end{tabular}
\end{table*}
